# Supplementary material for: Neural-Symbolic Logic Query Answering in Non-Euclidean Space
Source: arXiv:2603.15633 source file (2026-02-25)
Supplement: Supplementary file 1 [file 009appendix.tex]

\begin{figure}[htbp]
    \centering
    \includegraphics[width=0.99\textwidth]{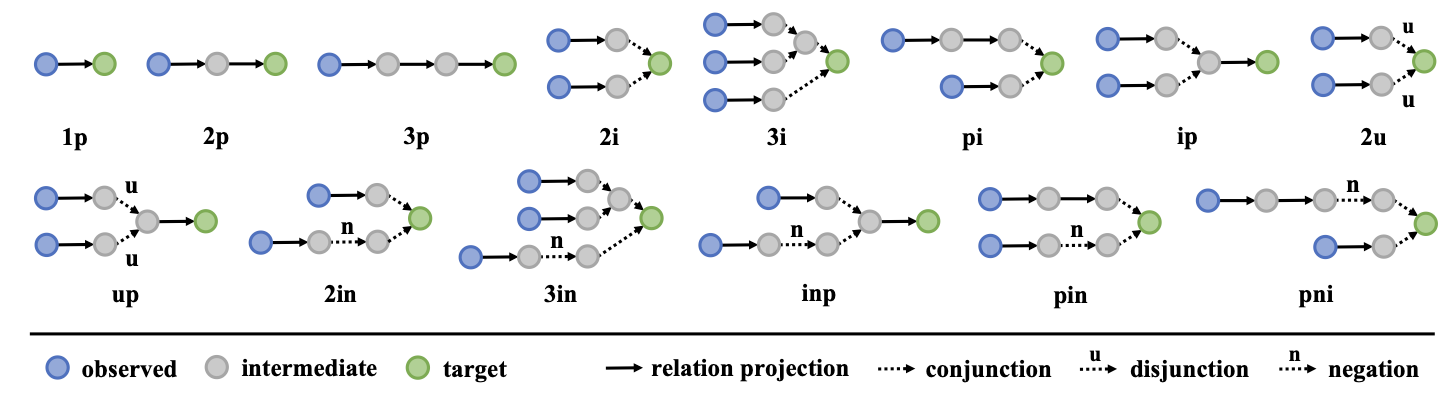}
    \caption{Types of complex FOL queries used in training and inference.}
    \label{fig:queries}
\end{figure}

We use the complex query datasets generated by (~\cite{query2box}). There is a total number of 14 query types, as showed in Figure ~\ref{fig:queries}. Statistics of all query types is summarized in Table. ~\ref{fig:queries_table}.

\begin{table}[ht]
\centering
\caption{Statistics of different query types used in the benchmark datasets.}
\begin{tabular}{|c|c|c|c|c|}
\hline
\textbf{Split} & \textbf{Query Type} & \textbf{FB15k} & \textbf{FB15k-237} & \textbf{NELL995} \\ \hline
Train & 1p/2p/3p/2i/3i & 273,710 & 149,689 & 107,982 \\ \hline
Train & 2in/3in/inp/pin/pni & 27,371 & 149,689 & 10,798 \\ \hline
Valid & 1p & 59,078 & 20,094 & 16,910 \\ \hline
Valid & Others & 8,000 & 5,000 & 4,000  \\ \hline
Test & 1p & 66,990 & 22,804 & 17,021 \\ \hline
Test & Others & 8,000 & 5,000 & 4,000 \\ \hline
\end{tabular}
\label{fig:queries_table}
\end{table}
